# Supplementary material for: Understanding the Effect of using Semantically Meaningful Tokens for Visual Representation Learning
Source: arXiv:2405.16401 source file (2025-05-19)
Supplement: Supplementary file 1 [file appendix.tex]

\appendix
\onecolumn

\setcounter{figure}{0}

\setcounter{table}{0} 

\section{Appendix}

\begin{figure}
    \centering
    \includegraphics{}
    \caption{\todo{figure to show which images benefit form our work. From COCO and ARO/Winoground}}
    \label{fig:compare_images}
\end{figure}
